# Supplementary material for: Efficient spin-wave excitation by surface acoustic waves in ultra-low damping YIG/ZnO-heterostructures
Source: arXiv:2503.11203 ancillary file (2025-03-14)
Supplement: Supplementary file 1 [file supplement.pdf]

# Efficient spin-wave excitation by surface acoustic waves in ultra-low damping YIG/ZnO-heterostructures

Yannik Kunz,[1,a)] Julian Schüler,[1] Finlay Ryburn,[2] Kevin Künstle,[1] Michael Schneider,[1] Katharina Lasinger,[1,2] Yangzhan Zhang,[2] Philipp Pirro,[1] John Gregg,[2] and Mathias Weiler[1]

[1)] *Fachbereich Physik and Landesforschungszentrum OPTIMAS, Rheinland-Pfälzische Technische Universität Kaiserslautern-Landau, 67663 Kaiserslautern, Germany*

[2)] *Clarendon Laboratory, Department of Physics, University of Oxford, Parks Road, Oxford, OX1 3PU, United Kingdom*

(Dated: 13 March 2025)

[a)] Electronic mail: ykunz@rptu.de

## I. SAMPLE PREPARATION

We use a 103 nm thin layer of yttrium-iron-garnet (YIG) which is grown via liquid-phase-epitaxy on a gadolinium gallium garnet (GGG). The zinc oxide (ZnO) is fabricated via sputtering deposition in an argon oxygen atmosphere at a ratio of 2:1 at a preassure of $4 \times 10^{-6}$ bar. After the sputtering, the sample is annealed in air for 6 h at 150 °C. The ZnO thickness is controlled via a calibrated deposition rate. The sets of interdigital transducers (IDTs) are fabricated by electron lithography and electron beam evaporation.

## II. DEFINITION OF THE SAW STRAIN COMPONENTS

We define the SAW strain composition by:

$$\varepsilon_{ij}(x,t) = \bar{\varepsilon}_{ij,0} \cdot e^{i(kx-\omega t)} \tag{1}$$

with $ij \in \{xx, xy, xz, yz\}$. Hereby, $\varepsilon_{ij,0}$ is the complex valued parametrization of the SAW component, with $\sqrt{\mathrm{Re}(\varepsilon_{ij,0})^2 + \mathrm{Im}(\varepsilon_{ij,0})^2}$ begin the amplitude and $\tan^{-1}(\mathrm{Im}(\varepsilon_{ij,0})/\mathrm{Re}(\varepsilon_{ij,0}))$ the phase. We provide the amplitude and phase of all strain components relative to the $xx$-component. The strain components are in approximation considered to be constant over the thickness in the YIG layer.

## III. FITTING PROCEDURE

In order to optimize the parameters used in the theoretical modeling in the main manuscript, we apply the following procedure. First, the magnetic parameters, determining the spin-wave dispersion relation, and thereby the angle-dependent resonance magnetic field, are optimized. For this, for each angle $\phi_H$ in the resonance magnetic field $\mu_0 H_{\mathrm{res}}$ of the minimum $\Delta S_{21}$-transmission is extracted. This is achieved by performing a parabolic fit in a confined region around the minima as to improve the accuracy. Next, the analytical solution for the resonance magnetic field as a function of the magnetic field orientation at

fixed frequency, is fitted using the expression:

$$\mu_0 H_{\mathrm{res}} = \frac{1}{2}\left(-\mu_0 H_{\mathrm{IP}} - \mu_0 H_{\mathrm{OOP}} + \sqrt{(\mu_0 H_{\mathrm{IP}} - \mu_0 H_{\mathrm{OOP}})^2 + \frac{16\pi f_0^2}{\gamma^2}}\right) \tag{2}$$

$$\mu_0 H_{\mathrm{OOP}} = \mu_0 G_0 M_{\mathrm{S}} - \frac{2K_{\mathrm{S}}}{M_{\mathrm{S}}} + \frac{2A}{M_{\mathrm{S}}}k^2 + \frac{2K_{\mathrm{u}}}{M_{\mathrm{S}}}\cos^2(\phi_H - \phi_{\mathrm{u}}) \tag{3}$$

$$\mu_0 H_{\mathrm{IP}} = \mu_0(1 - G_0)M_{\mathrm{S}}\sin^2(\phi_H) + \frac{2A}{M_{\mathrm{S}}}k^2 + \mu_0 H_{\mathrm{ani}}\cos(2(\phi_H - \phi_{\mathrm{u}})) \tag{4}$$

Here, $f_0$ is the frequency of the SAW, $\gamma$ the gyromagnetic ration, $G_0 = (1-\exp(-\|kt\|)/(kd)$ is the expression for the dipolar fields[1], $k$ is the wave vector, $d$ is the thickness of the ferromagnetic layer, $M_{\mathrm{S}}$ the saturation magnetization, $K_{\mathrm{S}}$ the OOP anisotropy constant, $K_{\mathrm{u}}$ the uniaxial anisotropy constant, $\phi_{\mathrm{u}}$ the uniaxial anisotropy easy axis and $A$ the exchange constant.

The fit of these parameters is carried out globally for the Rayleigh-mode and the Sezawa-mode at their distinct frequencies. Next, the Colormap data is fitted. For this, for each angle a subset around the resonance is used. Then, the strain parameters and the effective Gilbert damping are fitted, using the calculation model presented in Appendix A in the main manuscript. Consecutively, the strain parameters are normalized and fixed, while in a second fit the effective Gilbert damping and an arbitrary scaling parameter is fitted. This procedure is carried out for both the Rayleigh- and the Sezawa-Mode.

For all fitting procedures, Matlabs *lsqcurvefit*-solver is used.

## REFERENCES

[1]B. A. Kalinikos and A. N. Slavin, J. Phys. C: Solid State Phys. **19**, 7013 (1986).
